# Supplementary material for: A minimal-length approach unifies rigidity in under-constrained materials
Source: arXiv:1809.01586 ancillary file (2019-01-24)
Supplement: Supplementary file 1 [file supplement.pdf]

# Supplemental Information

A minimal-length approach unifies rigidity in under-constrained materials

Matthias Merkel,[1] Karsten Baumgarten,[2] Brian P. Tighe,[2] and M. Lisa Manning[1]

[1] *Department of Physics, Syracuse University, Syracuse, New York 13244, USA*

[2] *Delft University of Technology, Process & Energy Laboratory, Leeghwaterstraat 39, 2628 CB Delft, The Netherlands*

## CONTENTS

I. The minimum length function $\ell_{\rm min}$ controls the material behavior 1

A. System energy in terms of average and standard deviation of the rescaled spring lengths 1

B. The coefficients $a_\ell$ and $a_a$ are properties of a self-stress 2

C. Geometric properties and energy 3

1. Without shear strain 3
2. Including shear strain 4

D. Shear stress and shear modulus 4

E. Isotropic stress and bulk modulus 5

F. Scaling exponents for 2D spring networks 6

G. Application to rheometer geometry 7

II. Numerical results 7

A. Rigidity is created by geometric incompatibility 7

B. 2D spring networks 8

C. 2D fiber networks without bending rigidity 8

D. System-size dependence of the geometric parameters 10

III. There is at most one self-stress in the 2D vertex model with $k_A = 0$ 10

IV. Numerical energy minimization 11

A. Definitions for shear strain $\gamma$ 11

B. 2D spring networks 11

C. 2D vertex model 12

D. 2D Voronoi model 12

E. 3D Voronoi model 12

References 12

## I. THE MINIMUM LENGTH FUNCTION $\ell_{\rm min}$ CONTROLS THE MATERIAL BEHAVIOR

### A. System energy in terms of average and standard deviation of the rescaled spring lengths

Here we derive Eqs. (2) and (5) in the main text, starting from Eq. (1), which we restate here:

$$e_{s2D} = \sum_i (l_i - l_{0i})^2. \tag{S1}$$

To derive Eq. (2), we first introduce the mean rescaled spring rest length $\ell_0$, together with the rescaled spring lengths $\ell_i$ and the weights $w_i$:

$$\ell_0 = \left[\frac{1}{N}\sum_i l_{0i}^2\right]^{1/2} \tag{S2}$$

$$\ell_i = \ell_0 \frac{l_i}{l_{0i}} \tag{S3}$$

$$w_i = \left[\frac{l_{0i}}{\ell_0}\right]^2. \tag{S4}$$

In this subsection, all sums are over all springs $i$ in the network. The rescaled spring length $\ell_i$ is the actual spring length *measured relative to its rest lengths* and rescaled by $\ell_0$. Combining Eqs. (S1), (S3), and (S4), we obtain Eq. (2) in the main text:

$$e_{s2D} = \sum_i w_i(\ell_i - \ell_0)^2. \tag{S5}$$

We now need to show that Eq. (S5) is the same as Eq. (5) in the main text, which reads:

$$e_{s2D} = N\left[(\bar{\ell} - \ell_0)^2 + \sigma_\ell^2\right] \tag{S6}$$

with the following definitions for the (weighted) average and standard deviation of the rescaled spring lengths $\ell_i$:

$$\bar{\ell} = \frac{1}{N}\sum_i w_i \ell_i \tag{S7}$$

$$\sigma_\ell = \left[\frac{1}{N}\sum_i w_i(\ell_i - \bar{\ell})^2\right]^{1/2}. \tag{S8}$$

To this end, we first use Eqs. (S4) and (S2) to obtain:

$$\sum_i w_i = N. \tag{S9}$$

This relation is then used to transform $\sigma_\ell^2$ by expanding the square inside of the sum:

$$\sigma_\ell^2 = \frac{1}{N}\sum_i w_i \ell_i^2 - 2\bar{\ell}\frac{1}{N}\sum_i w_i \ell_i + \bar{\ell}^2, \tag{S10}$$

and with Eq. (S7):

$$\sigma_\ell^2 = \frac{1}{N}\sum_i w_i \ell_i^2 - \bar{\ell}^2. \tag{S11}$$

Adding $(\bar{\ell}-\ell_0)^2$ on both sides yields

$$(\bar{\ell}-\ell_0)^2+\sigma_\ell^2=\frac{1}{N}\sum_i w_i\ell_i^2-2\bar{\ell}\ell_0+\ell_0^2, \tag{S12}$$

and using again Eq. (S7):

$$(\bar{\ell}-\ell_0)^2+\sigma_\ell^2=\frac{1}{N}\sum_i w_i(\ell_i-\ell_0)^2. \tag{S13}$$

Hence, Eqs. (2) and (5) in the main text are equivalent.

### B. The coefficients $a_\ell$ and $a_a$ are properties of a self-stress

Here we show that the coefficients $a_\ell$ and $a_a$ are closely related to the self-stress $\boldsymbol{t}$ that is created at the onset of geometric incompatibility, at $\ell_0=\ell_0^*$ [1]. To this end, we start here by focusing on the case without area term, and where all weights are $w_i=1$ (cf. Eq. (2) in main text). At the end, we explain how to include both heterogeneous weights and area terms. Also, we assume for simplicity that close to the transition point there is only a single self-stress, which is the self-stress created by the onset of geometric incompatibility. However, while some models can only exhibit at most a single self-stress (Section III), we have convinced ourselves that our derivation can also be generalized to the case where several self-stresses are present at $\ell_0^*$. Finally, we assume here that there are no prestresses in the floppy regime, which implies that all lengths attain their preferred value right at the transition point. At the end of this section, we briefly discuss exceptions to this assumption. For clarity, we set $\gamma=0$ throughout this section.

A self-stress $\boldsymbol{t}$ is defined by

$$\boldsymbol{t}\cdot\boldsymbol{C}=0, \tag{S14}$$

where $\boldsymbol{C}$ is the compatibility matrix with components $C_{in}=\partial\ell_i/\partial r_n$, with $i=1,\ldots,N$ running over all generalized springs with lengths $\ell_i$, and $n$ running over all degrees of freedom $r_n$.

We show here that the creation of a self-stress $\boldsymbol{t}$ at the transition implies a linear scaling of the minimal average length $\bar{\ell}$ with $\sigma_\ell$. Moreover, it even implies such a scaling for each individual spring length $\ell_i$. To show this, we first note that – up to a prefactor – any vector $\boldsymbol{t}$ can always be written as:

$$\boldsymbol{t}=\boldsymbol{e}+a_\ell\boldsymbol{m}_t, \tag{S15}$$

where $\boldsymbol{e}=(1,\ldots,1)$ and $\boldsymbol{m}_t$ is some vector normalized such that $\boldsymbol{m}_t^2=N$ that is perpendicular to $\boldsymbol{e}$: $\boldsymbol{e}\cdot\boldsymbol{m}_t=0$. Thus, the coefficient $a_\ell$ represents here the ratio between standard deviation and average of the components $t_i$.

Given the existence of this self-stress, we are interested in the minimal possible average length $\bar{\ell}$ for fixed $\sigma_\ell$.

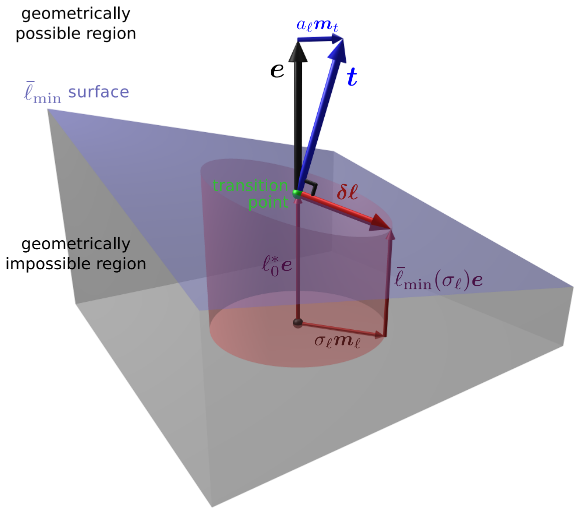


FIG. S1. Schematic illustrating the relation between the minimal length $\bar{\ell}_{\min}$ hyper-surface (blue surface) and the self-stress $\boldsymbol{t}$ (thick blue arrow) that is created at the onset of geometric incompatibility. Here, we show a 3D representation of the $N$-dimensional hyperspace containing all rescaled spring lengths $\boldsymbol{\ell}=(\ell_1,\ldots,\ell_N)$. The space is rotated such that the axis pointing up corresponds to the average spring length, i.e. it is parallel to the vector $\boldsymbol{e}=(1,\ldots,1)$ (black arrow). The horizontal plane in the image represents the remaining $N-1$ dimensions in the $\boldsymbol{\ell}$ space. The blue $\bar{\ell}_{\min}$ surface separates a geometrically possible region above it from a region of geometrically impossible spring length combinations $\boldsymbol{\ell}$ below it. Setting the spring rest lengths to the latter combinations will thus lead to geometric incompatibility and thus potentially rigidify the network. Close to the transition point (green sphere), the $\bar{\ell}_{\min}$ surface is perpendicular to the self-stress $\boldsymbol{t}$ (blue arrow), as expressed by Eq. (S18). The black sphere marks the point where all spring lengths are zero, and at the transition point (green sphere), all springs attain the same length $\boldsymbol{\ell}=\ell_0^*\boldsymbol{e}$. The distance from the line connecting both black and green points corresponds to the standard deviation of the spring lengths $\sigma_\ell$ (with a prefactor of $\sqrt{N}$). Hence, to obtain the minimal average length $\bar{\ell}_{\min}$ for given $\sigma_\ell$, we need to cut the mantle of a cylinder with radius $\sqrt{N}\sigma_\ell$ (red cylinder) with the $\bar{\ell}_{\min}$ surface. As we show via Eq. (S19), the resulting ellipse has its lowest point where $\boldsymbol{m}_\ell\uparrow\uparrow\boldsymbol{m}_t$. This figure corresponds to the case without area term. Also, this discussion relates to a local environment of one transition point. We expect that large displacements of the degrees of freedom $\boldsymbol{r}$ will affect this diagram by changing the direction of $\boldsymbol{m}_t$ (and by slightly altering the values of $\ell_0^*$ and $a_\ell$).

Similar to $\boldsymbol{t}$, we express the vector $\boldsymbol{\ell}$ containing all spring lengths as:

$$\boldsymbol{\ell}=\bar{\ell}\boldsymbol{e}+\sigma_\ell\boldsymbol{m}_\ell, \tag{S16}$$

where again $\boldsymbol{m}_\ell$ is a vector perpendicular to $\boldsymbol{e}$ normalized such that $\boldsymbol{m}_\ell^2=N$. Right at the transition point $\ell_0=\ell_0^*$, all lengths attain their preferred value $\boldsymbol{\ell}=\ell_0^*\boldsymbol{e}$. As we slightly decrease the control parameter $\ell_0$ by $\delta\ell_0$, and thus move into the rigid regime, the degrees of freedom will change by $\boldsymbol{\delta r}$. To first order in $\delta\ell_0$ this creates a

change in $\boldsymbol{\ell}$ by

$$\boldsymbol{\delta\ell} = \boldsymbol{C} \cdot \boldsymbol{\delta r}, \tag{S17}$$

where $\boldsymbol{\delta\ell} = (\bar{\ell} - \ell_0^*)\boldsymbol{e} + \sigma_\ell \boldsymbol{m}_\ell$. To minimize $\bar{\ell}$ for fixed $\sigma_\ell$, we need to take into account that $\boldsymbol{\delta\ell}$ can not attain any vector in its $N$-dimensional vector space. In particular, the existence of the self-stress $\boldsymbol{t}$ implies that $\boldsymbol{\delta\ell}$ has to be perpendicular to $\boldsymbol{t}$ (using Eqs. (S14) and (S17)):

$$\boldsymbol{t} \cdot \boldsymbol{\delta\ell} = 0. \tag{S18}$$

This equation is essentially a linearized version of the geometric compatibility condition $\bar{\ell} \geq \bar{\ell}_{\min}(\sigma_\ell)$. Note that Eq. (S18) is the only constraint when minimizing $\bar{\ell}$, besides fixing $\sigma_\ell$, because $\boldsymbol{t}$ is the only self-stress. Inserting Eq. (S15) and $\boldsymbol{\delta\ell}$ into Eq. (S18) yields:

$$\bar{\ell} = \ell_0^* - a_\ell \sigma_\ell (\boldsymbol{m}_t \cdot \boldsymbol{m}_\ell / N). \tag{S19}$$

The minimal $\bar{\ell}$ is obtained for $\boldsymbol{m}_\ell = \boldsymbol{m}_t$, where the scalar product $\boldsymbol{m}_t \cdot \boldsymbol{m}_\ell$ attains its maximal possible value $N$. Thus:

$$\bar{\ell}_{\min}(\sigma_\ell) = \ell_0^* - a_\ell \sigma_\ell. \tag{S20}$$

Insertion into Eq. (S16) yields:

$$\boldsymbol{\ell}(\sigma_\ell) = (\ell_0^* - a_\ell \sigma_\ell)\boldsymbol{e} + \sigma_\ell \boldsymbol{m}_t. \tag{S21}$$

Hence, also each individual spring length depends linearly on $\sigma_\ell$.

This proof is schematically illustrated by Fig. S1, where the $N$-dimensional space of spring lengths $\boldsymbol{\ell}$ is represented by a 3D figure. As for Eq. (S18), the $\bar{\ell}_{\min}$ surface (blue surface) is locally perpendicular to the self-stress $\boldsymbol{t}$ (blue arrow). In order to find the minimal possible $\bar{\ell}$ for given standard deviation $\sigma_\ell$, we first cut the $\bar{\ell}_{\min}$ surface with the locus where the standard deviation $\sigma_\ell$ has a defined constant value, which is a cylinder mantle (red). The cut is an ellipse, and as we show through Eq. (S19), its lowest point is where $\boldsymbol{m}_\ell \upuparrows \boldsymbol{m}_t$. Because the radius of the cylinder is proportional to $\sigma_\ell$, and because the blue $\bar{\ell}_{\min}$ surface is locally linear, we obtain that indeed $\ell_0^* - \bar{\ell}_{\min}(\sigma_\ell) \sim \sigma_\ell$.

To take heterogeneities in the weights $w_i$ into account, one can completely follow the above line of argument, where only the formal definition of the scalar product in the $N$-dimensional "constraint space" needs to be changed. In particular, the scalar product between two $N$-dimensional vectors $\boldsymbol{p}$ and $\boldsymbol{q}$ needs to be defined as:

$$\boldsymbol{p} \cdot \boldsymbol{q} = \sum_i w_i p_i q_i. \tag{S22}$$

Consequentially, also averages and standard deviations change, e.g. $\bar{t} = \boldsymbol{e} \cdot \boldsymbol{t}/N = [\sum_i w_i t_i]/N$ and $\sigma_t^2 = (\boldsymbol{t} - \bar{t}\boldsymbol{e})^2/N = [\sum_i w_i (t_i - \bar{t})^2]/N$.

For the cellular models with area term, the line of argument is similar, but with the following changes: First, vectors in the "constraint space" like the self-stress $\boldsymbol{t}$ now contain $2N$ components (where $N$ is the number of cells): $N$ of these components represent cell "lengths" and the other $N$ components represent cell "areas". Second, because the overall area is constant, there is a second self-stress where the length components are zero and the area components are one: $(0, \ldots, 0, 1, \ldots, 1)$. However, the important self-stress is still $\boldsymbol{t}$, which is now written as $\boldsymbol{t} = \boldsymbol{e} + a_\ell \boldsymbol{m}_t^\ell + a_a \boldsymbol{m}_t^a$, where $\boldsymbol{e} = (1, \ldots, 1, 0, \ldots, 0)$, the vector $\boldsymbol{m}_t^\ell$ has only non-zero length entries, and the vector $\boldsymbol{m}_t^a$ has only non-zero area entries. Consequentially, minimization of $\bar{\ell}$ for fixed $\sigma_\ell$ and $\sigma_a$ yields: $\bar{\ell}_{\min}(\sigma_\ell, \sigma_a) = \ell_0^* - a_\ell \sigma_\ell - a_a \sigma_a$.

Here we have assumed that at at the transition point $\ell_0 = \ell_0^*$, all spring lengths attain their preferred value $\ell_i = \ell_0^*$. In Section II A we numerically show that this is the case is nearly all of our models. However, it is in principle possible that this is not the case, but only if there are prestresses in the floppy regime, which we occasionally observed for the 2D vertex model with $k_A > 0$ (Fig. S4) and the 3D Voronoi model with $k_V > 0$ [2]. While we consider these exceptions outside the scope of the current paper, the above derivation can easily be generalized to obtain a formula for $\bar{\ell}_{\min}$ that includes these cases.

## C. Geometric properties and energy

Here we show how for all studied models, the function $\bar{\ell}_{\min}(\sigma_\ell, \sigma_a, \gamma)$ controls the behavior of the system in the rigid regime. In particular, knowing the functional form of $\bar{\ell}_{\min}(\sigma_\ell, \sigma_a, \gamma)$ lets us write explicit expressions for $\bar{\ell}$, $\sigma_\ell$, $\sigma_a$, and the total system energy $e$ in terms of the control parameters $k_A$, $\ell_0$, and $\gamma$.

### 1. *Without shear strain*

For all models, the dimensionless system energy $e$ can be expressed in terms of $\bar{\ell}$, $\sigma_\ell$, and $\sigma_a$:

$$e = N\Big[(\bar{\ell} - \ell_0)^2 + \sigma_\ell^2 + k_A \sigma_a^2\Big]. \tag{S23}$$

Because in the rigid regime, the average length attains the minimally possible length given $\sigma_\ell$ and $\sigma_a$, the energy minimum fulfills the following two equations:

$$0 = \frac{\partial e\Big(\bar{\ell} = \bar{\ell}_{\min}(\sigma_\ell, \sigma_a), \sigma_\ell, \sigma_a\Big)}{\partial \sigma_\ell} \tag{S24}$$

$$0 = \frac{\partial e\Big(\bar{\ell} = \bar{\ell}_{\min}(\sigma_\ell, \sigma_a), \sigma_\ell, \sigma_a\Big)}{\partial \sigma_a}. \tag{S25}$$

Insertion of Eq. (S23) yields:

$$\sigma_\ell = -\frac{\partial \bar{\ell}_{\min}}{\partial \sigma_\ell}(\bar{\ell} - \ell_0) \tag{S26}$$

$$\sigma_a = -\frac{1}{k_A}\frac{\partial \bar{\ell}_{\min}}{\partial \sigma_a}(\bar{\ell} - \ell_0). \tag{S27}$$

If we knew the relation $\bar{\ell}_{\min}(\sigma_\ell, \sigma_a)$, we could just insert it together with $\bar{\ell} = \bar{\ell}_{\min}$ into Eqs. (S26) and (S27) in order to obtain explicit expressions for $\bar{\ell}$, $\sigma_\ell$, and $\sigma_a$ depending on the control parameters $\ell_0$ and $k_A$.

For example, close to the transition point we find that $\bar{\ell}_{\min}(\sigma_\ell, \sigma_a)$ depends linearly on $\sigma_\ell$ and $\sigma_a$:

$$\bar{\ell}_{\min}(\sigma_\ell, \sigma_a) = \ell_0^* - a_\ell \sigma_\ell - a_a \sigma_a. \tag{S28}$$

This is a consequence of the self-stress that is created at the onset of rigidity (see Section I B). Insertion into Eqs. (S26) and (S27) yields:

$$\sigma_\ell = a_\ell(\bar{\ell} - \ell_0) \tag{S29}$$

$$\sigma_a = \frac{a_a}{k_A}(\bar{\ell} - \ell_0). \tag{S30}$$

Further, using again Eq. (S28), we obtain:

$$\bar{\ell} = \ell_0 + \frac{1}{Z}(\ell_0^* - \ell_0) \tag{S31}$$

$$\sigma_\ell = \frac{a_\ell}{Z}(\ell_0^* - \ell_0) \tag{S32}$$

$$\sigma_a = \frac{a_a}{k_A Z}(\ell_0^* - \ell_0) \tag{S33}$$

with

$$Z = 1 + a_\ell^2 + \begin{cases} 0 & \text{for } k_A = 0, \text{ and} \\ \frac{a_a^2}{k_A} & \text{for } k_A > 0. \end{cases} \tag{S34}$$

Finally, inserting Eqs. (S31)–(S33) into Eq. (S23), we obtain an explicit expression of $e$ in terms of the control parameters $\ell_0$ and $k_A$:

$$e = \frac{N}{Z}(\ell_0^* - \ell_0)^2, \tag{S35}$$

where $Z$ depends on $k_A$ according to Eq. (S34).

#### 2. *Including shear strain*

The minimal length function generally depends also on the shear strain $\gamma$. Note that in our formalism there are no requirements on the precise definition of $\gamma$, which can in particular describe any of both pure shear or simple shear deformation. Please refer to Section IV for the precise definition of $\gamma$ used in each of the studied models.

We assume that $\bar{\ell}_{\min}(\sigma_\ell, \sigma_a, \gamma)$ is analytic in $\gamma$, and close to the transition, we can thus write up to first order in $\sigma_\ell$ and $\sigma_a$ and up to second order in $\gamma$:

$$\bar{\ell}_{\min}(\sigma_\ell, \sigma_a, \gamma) = \ell_0^* - a_\ell \sigma_\ell - a_a \sigma_a + b\gamma^2. \tag{S36}$$

Note that there is some freedom in choosing the point $\gamma = 0$, which allows us to discard the linear term $\sim \gamma$ in Eq. (S36). This point is automatically reached by searching for the point $\ell_0 = \ell_0^*$ and $\gamma = 0$ using a shear-stabilized minimization protocol for simulations [3], or in experiments by starting from a stress-free state with minimal $\ell_0$ (Section I D). Moreover, generally there are of course also terms $\sim \sigma_{\ell/a}\gamma$ and $\sim \sigma_{\ell/a}\gamma^2$. These terms allow to predict higher-order corrections to the energy and its derivatives. However, for this study we focus just on the highest-order terms as listed in Eq. (S36).

Following the same arguments as in the previous subsection, we ultimately obtain for the system energy:

$$e = \frac{N}{Z}\left(\ell_0^* - \ell_0 + b\gamma^2\right)^2, \tag{S37}$$

where $Z$ is again given by Eq. (S34). In the following Sections I D and I E below we compute several derivatives of this expression to obtain the mechanical material properties.

### D. Shear stress and shear modulus

Using the expression Eq. (S37), we obtain the following expression for the shear stress $\tilde{\sigma} = (\mathrm{d}e/\mathrm{d}\gamma)/N$ in the rigid regime, with $N$ being the dimensionless system area:

$$\tilde{\sigma} = \frac{4b\gamma}{Z}\left(\ell_0^* - \ell_0 + b\gamma^2\right). \tag{S38}$$

Note that a term $\sim \gamma$ in $\ell_{\min}$ (Eq. (S36)) would lead to an additional constant term in the numerator of Eq. (S38). Thus, the shear stress for $\ell_0 < \ell_0^*$ would be nonzero at $\gamma = 0$.

From Eq. (S38), we obtain the differential shear modulus $G = \mathrm{d}\tilde{\sigma}/\mathrm{d}\gamma$ in the rigid regime:

$$G = \frac{4b}{Z}\left(\ell_0^* - \ell_0 + 3b\gamma^2\right). \tag{S39}$$

Combining this with Eq. (S38), we obtain:

$$G = \Delta G^* + \frac{3\tilde{\sigma}}{\gamma}, \tag{S40}$$

where $\Delta G^*$ is:

$$\Delta G^* = \frac{8b}{Z}(\ell_0 - \ell_0^*). \tag{S41}$$

This is the shear modulus discontinuity in $G$, which appears at the onset of rigidity $\gamma = \gamma^*$.

For $\gamma = 0$ and $\ell_0 < \ell_0^*$, Eq. (S39) implies that the shear modulus $G$ scales linearly with the distance $\ell_0^* - \ell_0$ to the transition point. This is confirmed by our model simulations for the 2D spring networks in Fig. 4f in the main text, and for the cellular models in Fig. S2, in part confirming earlier findings [2, 4, 5]. Fig. S2 also shows a collapse of the different $k_A > 0$ curves of a given model when rescaling the shear modulus with $Z$, indicating that $b$ indeed describes the underlying geometry and is thus independent of $k_A$. However, note that like the coefficients $a_\ell$, also the coefficient $b$ may differ between the $k_A = 0$ and $k_A > 0$ versions of a model (see in particular

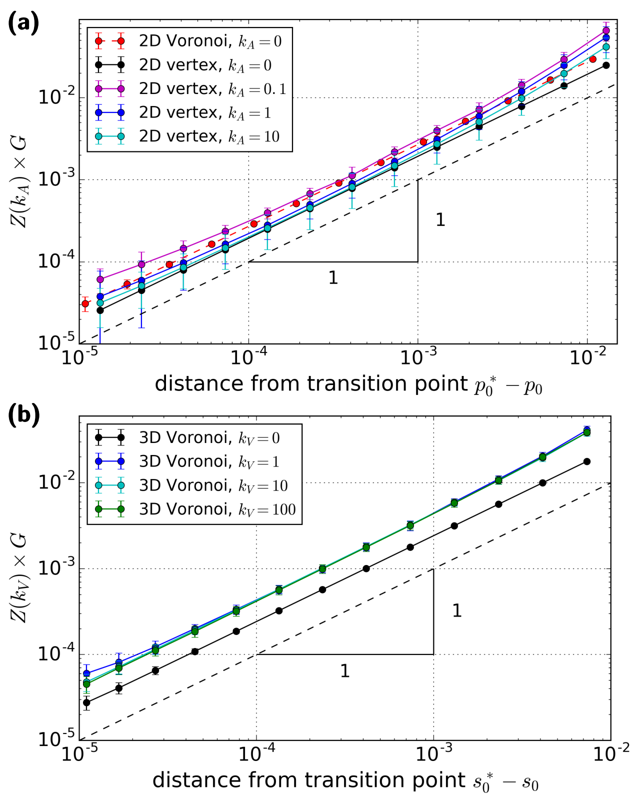


FIG. S2. For $\gamma = 0$ and $\ell_0 < \ell_0^*$, the shear modulus $G$ scales linearly with the distance $\ell_0^* - \ell_0$ to the transition point (cf. Eq. (S39)). (a) 2D Voronoi and 2D vertex model, (b) 3D Voronoi model. Rescaling the shear modulus by $Z$ defined in Eq. (S34) largely collapses the data for all $k_A > 0$ values of a given model.

Fig. S2b). The reason is that they represent Taylor expansions of the function $\bar{\ell}_{\min}(\sigma_\ell, \sigma_a, \gamma)$ at different points $(\sigma_\ell, \sigma_a, \gamma)$. For $k_A > 0$, the coefficient $b$ characterizes the behavior at $(\sigma_\ell, \sigma_a, \gamma) = (0, 0, 0)$, while for $k_A = 0$ at $(\sigma_\ell, \sigma_a, \gamma) = (0, \sigma_a > 0, 0)$. The numerical values of $b$ are noted in Table I in the main text.

### E. Isotropic stress and bulk modulus

In order to derive the isotropic part of the stress and the bulk modulus from the energy expression Eq. (S37), we make use of the fact that $\ell_0$ is non-dimensionalized by the number density of elements, and thus indirectly depends on the system size.

To make sure we are not missing any term, we start from the “dimensionful” energy of the system, which reads:

$$E = \sum_i \left[ K_L (L_i - L_0)^2 + K_A (A_i - A_0)^2 \right]. \qquad \text{(S42)}$$

Here, $K_L$ and $K_A$ are length and area rigidities, $L_i$ and $A_i$ are length and area of element $i$, and $L_0$ and $A_0$ are their respective preferred values. Thus, the total area of the system is $A_T = \sum_i A_i$ and the average area per element is $\bar{A} = A_T/N$. To obtain the dimensionless expressions $e$ for the energies of our models (Eqs. (1)–(4) in the main text), we have set $A_0 = \bar{A}$ and then non-dimensionalized with respect to the length scale $\bar{A}^{1/D}$ and the energy scale $K_L \bar{A}^{2d/D}$ [2, 6, 7]. Hence, the dimensionful total energy $E$ of the system can be written as the sum:

$$E = E_{A_0} + K_L \bar{A}^{2d/D} e, \qquad \text{(S43)}$$

where $E_{A_0} = N K_A (\bar{A} - A_0)^2$ is a mean-field contribution by the area elasticity, and $e$ is the non-dimensional energy given by Eq. (S37).

The isotropic part of the stress is defined as the negative (dimensionful) pressure $-P = \mathrm{d}E/\mathrm{d}A_T = (\mathrm{d}E/\mathrm{d}\bar{A})/N$. Insertion of Eq. (S43) yields:

$$-P = 2K_A(\bar{A} - A_0) + \frac{K_L \bar{A}^{2d/D}}{N} \left[ \frac{2d}{D\bar{A}} e + \frac{\mathrm{d}e}{\mathrm{d}\bar{A}} \right]. \qquad \text{(S44)}$$

We obtain for the dimensionless pressure $p = \bar{A}^{1-2d/D} P / K_L$:

$$-p = 2k_A(1 - a_0) + \frac{1}{N} \left[ \frac{2d}{D} e + \bar{A} \frac{\mathrm{d}e}{\mathrm{d}\bar{A}} \right] \qquad \text{(S45)}$$

with $a_0 = A_0/\bar{A}$.

While in the floppy regime the dimensionless energy $e$ is zero, in the rigid regime $e$ is given by Eq. (S37) in terms of shear strain $\gamma$ and the dimensionless control parameters $k_A = K_A \bar{A}^{2-2d/D}/K_L$ and $\ell_0 = L_0/\bar{A}^{d/D}$. The derivatives of $k_A$ and $\ell_0$ with respect to $\bar{A}$ are:

$$\frac{\mathrm{d}k_A}{\mathrm{d}\bar{A}} = \frac{2(D-d)k_A}{D\bar{A}} \qquad \frac{\mathrm{d}\ell_0}{\mathrm{d}\bar{A}} = -\frac{d\ell_0}{D\bar{A}}. \qquad \text{(S46)}$$

Hence, we ultimately obtain for the pressure $p$ to first order in $\ell_0^* - \ell_0 + b\gamma^2$ and for $b\gamma^2 \ll \ell_0^*$:

$$-p = 2k_A(1 - a_0) + \frac{2d\ell_0^*}{DZ} (\ell_0^* - \ell_0 + b\gamma^2). \qquad \text{(S47)}$$

Comparison with the shear modulus $G$, Eq. (S39), for $k_A = 0$ or $a_0 = 1$ yields the second relation in Eq. (13) in the main text.

From Eq. (S47) directly follows that the Poynting coefficient $\chi = p/\gamma^2$ close to $\ell_0 = \ell_0^*$ is for $k_A = 0$ or $a_0 = 1$:

$$\chi = -\frac{2db\ell_0^*}{DZ}. \qquad \text{(S48)}$$

For 2D spring networks, this prediction is tested in Fig. S5b & inset.

The bulk modulus is defined by $-A_T(\mathrm{d}P/\mathrm{d}A_T) = -\bar{A}(\mathrm{d}P/\mathrm{d}\bar{A})$, and thus the dimensionless bulk modulus is

$$B = -\frac{\bar{A}^{2-2d/D}}{K_L} \frac{\mathrm{d}P}{\mathrm{d}\bar{A}}. \qquad \text{(S49)}$$

Insertion of the pressure $P$, Eq. (S44), yields in the floppy regime:

$$B = 2k_A, \tag{S50}$$

and in the rigid regime:

$$B = 2k_A + \frac{1}{N}\left[\frac{2d(2d-D)}{D^2}e + \frac{4d}{D}\bar{A}\frac{\mathrm{d}e}{\mathrm{d}\bar{A}} + \bar{A}^2\frac{\mathrm{d}^2 e}{\mathrm{d}\bar{A}^2}\right]. \tag{S51}$$

To absolute order in $\ell_0^* - \ell_0 + b\gamma^2$ and for $\gamma = 0$, only the last term in the square brackets survives when inserting Eq. (S37):

$$B = 2k_A + \frac{2d^2(\ell_0^*)^2}{D^2 Z}. \tag{S52}$$

This is the bulk modulus when approaching the transition from the rigid regime. To extend this expression for $\gamma \neq 0$ and into the rigid regime $\ell_0^* - \ell_0 + b\gamma^2 > 0$, higher order terms in $\bar{\ell}_{\mathrm{min}}$ need to be taken into account. Note that Eq. (S52) can also be derived by projecting the affine isotropic deformation mode onto the self-stress $\boldsymbol{t}$ that is created at the onset of geometric incompatibility (Section I B) [1].

The prefactor $Z$ in Eq. (S52), and thus ultimately the coefficients $a_\ell$ and $a_a$ (Eq. (S34)), represent the effect of non-affinities during isotropic deformations. To see this, consider a system at the transition point, where all dimensionless areas are $a_i = 1$ and all dimensionless lengths are $\ell_i = \ell_0^*$. An *affine* isotropic deformation starting from this configuration means that all dimensionless $a_i$ and $\ell_i$ stay the same, because we non-dimensionalize with the average area $\bar{A}$. With Eq. (S23) follows that the energy for affine transformations away from the transition point towards the solid regime would then be $e = N(\ell_0^* - \ell_0)^2$. The difference to Eq. (S37) is just the prefactor $Z^{-1}$, which thus indeed accounts for the non-affinities.

### F. Scaling exponents for 2D spring networks

Here we rationalize for the 2D spring networks the observed approximate scaling exponents in the coefficients $a_\ell \sim \Delta z^{1/2}$ (Fig. 2a inset in the main text) and $b \sim \Delta z$ (Fig. 4c inset in the main text).

To understand the scaling of the coefficient $a_\ell$, we start with the extended Hessian $\boldsymbol{H}_\lambda$ of the system, which we define as the second energy derivative with respect to both, all internal degrees of freedom $r_n$ *and a global linear scaling factor* $\lambda$. We denote the eigen frequencies of this extended Hessian by $(\omega_\lambda^m)^2$ and the $\lambda$ component of the corresponding eigen vectors by $\Lambda_\lambda^m$. Then, the bulk modulus $B = (\mathrm{d}^2E/\mathrm{d}\lambda^2)/D^2N$ can be expressed using the well-known formula [2, 8, 9]:

$$\left[\frac{\mathrm{d}^2 E}{\mathrm{d}\lambda^2}\right]^{-1} = \sum_m \frac{(\Lambda_\lambda^m)^2}{(\omega_\lambda^m)^2}. \tag{S53}$$

We use this formula in the rigid regime approaching the transition. In this case, there are many low-frequency modes, which correspond to the zero modes in the floppy regime. However, as evidenced by the bulk modulus discontinuity, these modes have vanishing $\lambda$ component [1, 2]: $\Lambda_\lambda^m = 0$. Thus, we can treat the quantities on the right-hand side of Eq. (S53) as those of the unstressed Hessian, ignoring any zero modes in the sum [2]. Insertion of Eq. (S52) and transforming the sum into an integral yields:

$$1 + a_\ell^2 \sim \int_{0+}^{\infty} \frac{D_\lambda(\omega)\Lambda_\lambda^2(\omega)}{\omega^2}\,\mathrm{d}\omega. \tag{S54}$$

Here $D_\lambda(\omega)$ is the density of states, and we used that $\ell_0^*$ is to dominant order independent of $\Delta z$ (Table I and Fig. 1b inset in main text). It has been shown that for the "non-extended" Hessian $\boldsymbol{H}$, the density of states $D$ shows a plateau starting at $\omega^* \sim \Delta z$ [10, 11]. Assuming that $\Lambda_\lambda$ does not depend strongly on $\omega$ and that $D_\lambda \simeq D$, we obtain

$$1 + a_\ell^2 \sim \frac{1}{\Delta z}. \tag{S55}$$

For $\Delta z \ll 1$ follows indeed that $a_\ell \sim \Delta z^{1/2}$. Deviations that we observe in our 2D system for small $\Delta z$ (Fig. 2a inset in the main text) may be related to logarithmic corrections [11].

We use a related argument to understand the scaling of the coefficient $b$. Now we use the Hessian $\boldsymbol{H}_\gamma$ extended by the shear strain $\gamma$. Analogously to above, we denote the eigen frequencies of this extended Hessian by $(\omega_\gamma^m)^2$ and the $\gamma$ component of the corresponding eigen vectors by $\Lambda_\gamma^m$. We use the analogous formula to Eq. (S53) for the shear modulus [2, 8, 9]:

$$\frac{1}{NG} = \sum_m \frac{(\Lambda_\gamma^m)^2}{(\omega_\gamma^m)^2}. \tag{S56}$$

Using Eqs. (S39) and (S47) with $\gamma = 0$, this equation can be transformed into

$$\frac{1}{b(-p)} \sim \int_{0+}^{\infty} \frac{D_\gamma(\omega)\Lambda_\gamma^2(\omega)}{\omega^2}\,\mathrm{d}\omega. \tag{S57}$$

Here, $-p$ is the isotropic stress acting on the boundaries of the system. The major difference to the isotropic case, Eq. (S54), is that the shear modulus *vanishes* when approaching the point $\ell_0 = \ell_0^*$ and $\gamma = 0$ from the rigid side. This means that right at the transition, there are zero modes of $D_\gamma$ with non-vanishing overlap $\Lambda_\gamma^m \neq 0$. As a consequence, in the rigid vicinity of the transition where $-p$ is small, the integral Eq. (S57) is dominated by these modes, which are raised to energies $\sim (-p)$ [2]. Indeed, some of us recently showed that for small $-p$, the product $D_\gamma\Lambda_\gamma^2$ collapses for different $\Delta z$ and $-p$ as [12]:

$$D_\gamma(\omega)\Lambda_\gamma^2(\omega)\,\mathrm{d}\omega = \Delta z f_\gamma(x)\,\mathrm{d}x \tag{S58}$$

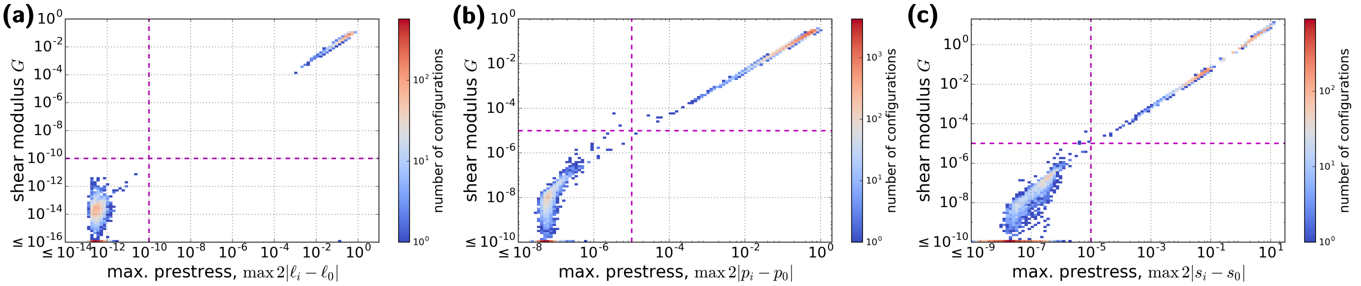


FIG. S3. Rigidity is created by geometric incompatibility. This is shown here by 2D histograms with respect to the largest prestress in a given configuration (directly indicating geometric incompatibility, $x$ axis) and its shear modulus ($y$ axis), for (a) 2D spring networks, here with $z = 3.2$, (b) the 2D vertex model with $k_A = 0$ and (c) the 3D Voronoi model with $k_V = 0$. Earlier publications have shown this for the 2D Voronoi model with $k_A = 0$ [7] and the 3D Voronoi model with $k_V > 0$ [2].

with $x = \omega/\sqrt{-p}$ and $f_\gamma$ being independent of $\Delta z$ and $p$. This makes sense, because at the transition there are $\sim \Delta z$ zero modes, which are all raised to energies $\sim (-p)$. Insertion of Eq. (S58) into Eq. (S57) yields:

$$\frac{1}{b(-p)} \sim \frac{\Delta z}{-p}, \tag{S59}$$

and thus $b \sim 1/\Delta z$. More details on the shear modulus scaling in the spring networks can be found in Ref. [12].

### G. Application to rheometer geometry

To facilitate the comparison of our results to experiments, we briefly discuss here how our results apply to a rheometer geometry with circumferential axis $x$, radial axis $y$, and rotation axis $z$, and the shear strain $\gamma$ corresponds to the simple shear strain. Rheometers typically measure shear stress $\tilde{\sigma} = \sigma_{xz}$ and normal stress $\sigma_{zz}$.

In the following, we show for that several experimental protocols, and in the vicinity of the $(\gamma, \ell_0) = (0, \ell_0^*)$ point, the normal stress $\sigma_{zz}$ should be dominated by the isotropic part of the stress tensor, $-p$, given by Eq. (S47). To this end, we will assume no lateral (i.e. radial) deformation of the network in the rheometer, which we expect to be valid whenever the sample is glued to the rheometer plates and its height is small as compared to its radius.

First, we expect the normal stress $\sigma_{zz}$ to be dominated by the isotropic stress, $\sigma_{zz} \simeq -p$, upon application of simple shear starting from a stress-free state. To show this, we use the Lodge-Meissner relation [13], which states that the normal stress difference is:

$$\sigma_{xx} - \sigma_{zz} = \tilde{\sigma}\gamma. \tag{S60}$$

Note that while this relation likely holds generally for isotropic, purely elastic materials, we consider a proof of this to be outside the scope of this article. Combined with Eqs. (S38) and (S47), we find:

$$\sigma_{xx} - \sigma_{zz} = -\frac{2Db\gamma^2}{d\ell_0^*}p. \tag{S61}$$

Hence, for $\gamma \ll 1$ we obtain that the normal stress difference is much smaller than the isotropic stress $-p$, and thus $\sigma_{zz} \simeq -p$.

We expect the same also for uniaxial compression or expansion of the sample along the $z$ axis [14]. This is because in the absence of lateral deformation, both isotropic strain and pure shear strain along the $z$ axis will have the same magnitude $\varepsilon$. When expanding the sample starting from $\ell_0 = \ell_0^*$, the discontinuity in the bulk modulus will lead to lowest order in $\varepsilon$ to a linear increase in the isotropic stress $-p \sim \varepsilon$. However, because of the linear increase of the shear modulus with $(\ell_0^* - \ell_0) \sim \varepsilon$, the normal stress difference will increase only as $\sim \varepsilon^2$. Hence, we find also for small uniaxial deformations: $\sigma_{zz} \simeq -p$.

## II. NUMERICAL RESULTS

### A. Rigidity is created by geometric incompatibility

Here we discuss numerical evidence showing that geometric incompatibility is both necessary and sufficient to create rigidity in the models studied. We have shown this before for the $k_V > 0$ case of the 3D Voronoi model [2] and for the $k_A = 0$ case for the 2D Voronoi model [7]. For the 2D spring networks, the 2D vertex model with $k_A = 0$, and the 3D Voronoi model with $k_V = 0$, we demonstrate this in Fig. S3.

In Fig. S3, we sorted all energy-minimized configurations into two-dimensional histograms with respect to the shear modulus $G$ and the maximal prestress $2|\ell_i - \ell_0|$ in the configuration. The dashed magenta lines indicate cutoff values below which we regard shear modulus and maximal prestress as numerically zero (obtained as described in [2]). The fact that the upper-left and lower-right quadrants in all three plots are essentially devoid of configurations means that geometric incompatibility is necessary and sufficient, respectively, to create rigidity in these models.

For the 2D vertex model with $k_A > 0$ we find exceptions to this, similar to the 3D Voronoi model with $k_V > 0$ [2]. Note that all results presented here are

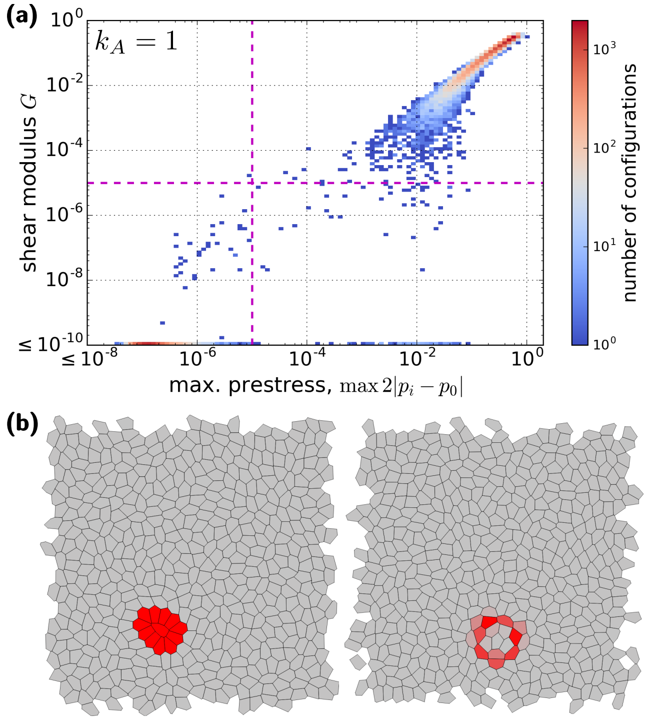


FIG. S4. In the 2D vertex model with $k_A > 0$, rigidity is created by the onset of geometric incompatibility, but there are also localized prestresses. (a) Geometric incompatibility is necessary for rigidity, and in many cases also sufficient. However, there were several energy-minimized configurations with finite prestresses, but vanishing shear modulus. (b) Two such configurations, with $p_0 = 3.939$ and $p_0 = 3.939$, respectively. The color of each cell $i$ indicates $p_i - p_0$, where gray corresponds to a value of zero and bright red to a value of 0.05. $k_A = 1$ in both panels. Shown here are only configurations without quadrilaterals (see Section IV).

based on configurations without quadrilaterals and triangles (see Section IV). Like for the other models, also for the 2D vertex model with $k_A > 0$ geometric incompatibility (i.e. the existence of prestresses) is *necessary* to create rigidity (i.e. a finite shear modulus). This is suggested by the essential absence of configurations in the upper-left quadrant in Fig. S4a. However, the existence of prestresses is not always *sufficient* to rigidify the system, as can be seen by the configurations in the lower-right quadrant of this plot. Examples for such configurations are shown in Fig. S4b, where the color indicates the value of $p_i - p_0$ of each cell, with gray indicating a value of zero and red indicating a positive value. The cells with finite perimeter tension are localized to one region and do not percolate the system. Note that when probing the scaling of $\ell_{\rm min}$ and of mechanical properties, we excluded networks with such localized prestresses (i.e. in Fig. 2b in the main text, Fig. S2a, and Fig. S7d-f).

## B. 2D spring networks

Here we report additional numerical results on the 2D spring networks. First, we found occasional jumps when probing the dependence of the critical shear strain $\gamma^*$ on $\ell_0 > \ell_0^*$ (see Fig. S5a for $z = 3.7$). We observed that these jumps occur more frequently for higher coordination number $z$, i.e. for systems closer to isostaticity. We interpret these jumps as plastic events where the system switches into the basin of a different minimum of $\ell_{\rm min}(0, \gamma)$. In particular, we numerically looked for the critical strain $\gamma^*$ by increasing $\gamma$ in steps of size $\Delta\gamma$ until the system rigidified (see Section IV). Notably, upon decreasing $\Delta\gamma$, we obtained less jumps in $\gamma^*$, consistent with a decreased probability of switching basins when taking smaller steps. Throughout this article, we focus on the purely elastic behavior of the system in the vicinity of one local minimum of $\bar{\ell}_{\rm min}(\sigma_\ell = 0, \gamma)$, and exclude these cases from our analysis.

Second, in the past, randomly-cut packing-derived spring networks have been studied without varying the parameter $\ell_0$, where instead the value $\ell_0^{\rm init}$ right after initialization of the spring network was used, e.g. in Ref. [15]. In order to compare to the scaling relations with respect to $\Delta z$ found in the past, we numerically studied the scaling of $\ell_0^{\rm init} - \ell_0^*$ and find that it scales as $(\ell_0^{\rm init} - \ell_0^*) \sim \Delta z$. Together with our other findings, we recapitulate indeed several of the scaling exponents observed in Ref. [15] (see discussion section in the main text).

Third, we also observe a negative Poynting effect, which is reflected in the development of a tensile isotropic stress $-p$ upon shear. For $\ell_0 = \ell_0^*$, the isotropic stress scales quadratically with the shear strain $\gamma$, which is shown in Fig. S5b for $z = 3.2$. Moreover, we can predict the corresponding coefficient $\chi = p/\gamma^2$ using Eq. (S48) by extracting the coefficient $b$ for each network from the scaling of the critical shear $\gamma^*$ with $\ell_0 > \ell_0^*$ (Fig. S5b inset).

Fourth, the existence of the function $\ell_{\rm min}$ allows the prediction not only of the Poynting coefficient $\chi$, but also of the coefficient describing the linear shear modulus scaling for $\ell_0 < \ell_0^*$ (Fig. S5c, cf. Fig. 4f) and of the shear modulus discontinuity (Fig. S5c inset, cf. Fig. 4d inset).

## C. 2D fiber networks without bending rigidity

We also simulated a fiber network model without bending rigidity. To this end, we divided each spring of our 2D spring networks into $M$ "subsprings" (Fig. S6a). These subspring networks are still under-constrained, and the limit $M \to \infty$ corresponds to fiber networks without bending rigidity. We find that such subspring networks also follow the predictions that we make in the main text (Fig. S6b-e, cf. Fig. 4 in the main text). Moreover, we also find numerically that these results are quantita-

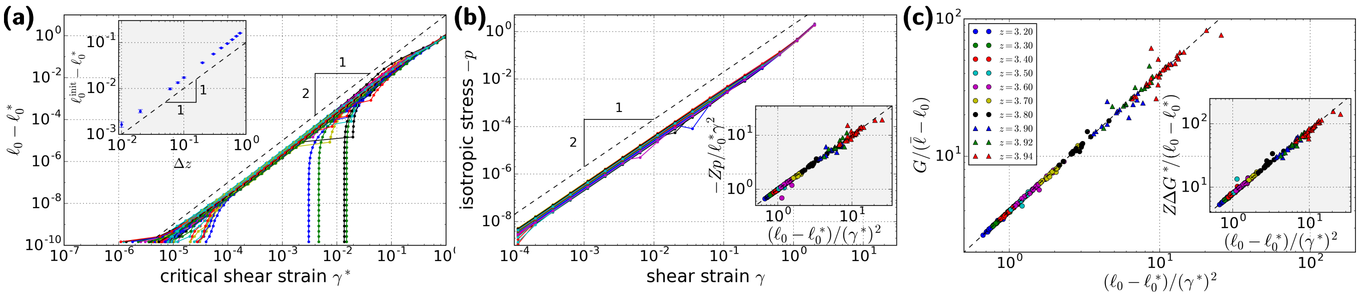


FIG. S5. Additional numerical results for the scaling in 2D spring networks. (a) Dependence of the critical shear $\gamma^*$ on $\ell_0 - \ell_0^*$ for $z = 3.7$ (cf. Fig. 4c in the main text). We interpret the jumps in $\gamma^*$ as a switch of the system into the basin of a different minimum of $\ell_{\rm min}(0, \gamma)$. (a inset) The value of $\ell_0$ right after creation of the spring network, $\ell_0^{\rm init}$, behaves such that we numerically observe the scaling relation $(\ell_0^{\rm init} - \ell_0^*) \sim \Delta z$. (b) Atypical negative Poynting effect: Quadratic scaling of the tensile isotropic stress $-p$ with the shear strain $\gamma$ for $\ell_0 = \ell_0^*$ and $z = 3.2$. (b inset) Prediction of the prefactor in panel b based on the scaling of the critical shear $\gamma^*$ with $\ell_0 - \ell_0^*$ for $\ell_0 > \ell_0^*$. The black dashed line represents the prediction according to Eq. (S48). (c) Prediction of the prefactor in the linear shear modulus scaling for $\ell_0 < \ell_0^*$ with $\gamma = 0$ based on the scaling of the critical shear $\gamma^*$ with $\ell_0 - \ell_0^*$ for $\ell_0 > \ell_0^*$. The black dashed line represents the prediction according to the relation $G = 4b(\bar{\ell} - \ell_0)$. (c inset) Prediction of the shear modulus discontinuity $\Delta G^*$ for $\ell_0 > \ell_0^*$ based on the scaling of the critical shear $\gamma^*$ with $\ell_0 - \ell_0^*$. The black dashed line represents the prediction according to Eq. (S41). In panel c and the insets to panels b and c, each symbol represents one probed spring network. In the insets to panels b and c, $Z$ was extracted from the geometric scaling of the respective networks for $\ell_0 < \ell_0^*$, using Eq. (S29).

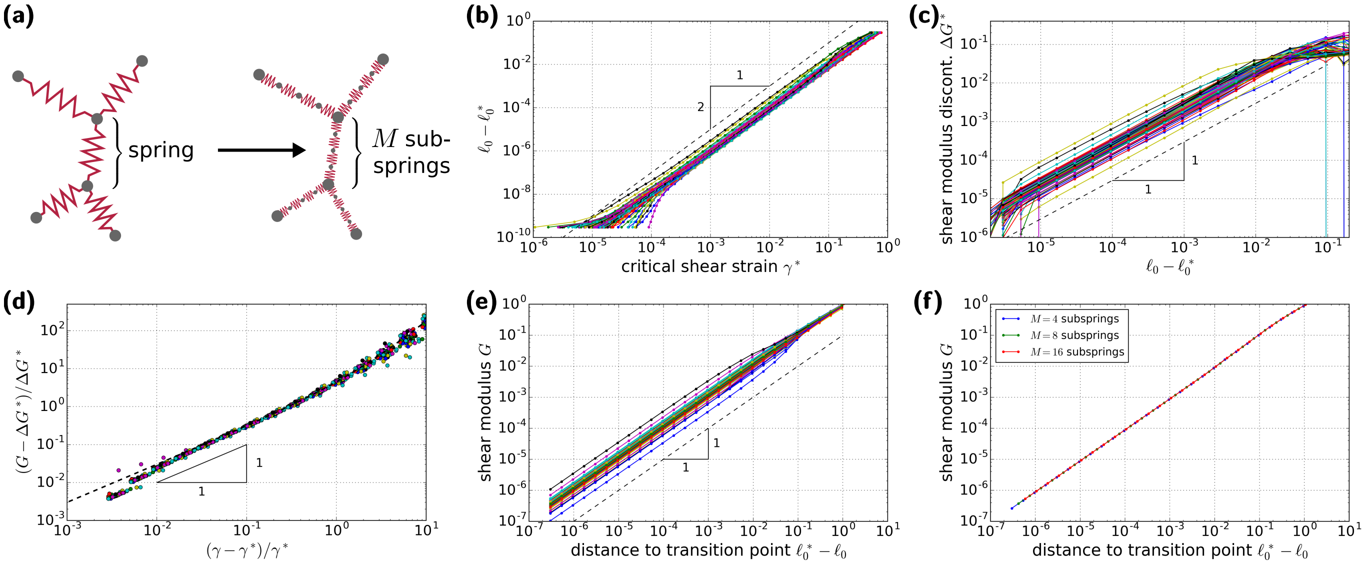


FIG. S6. Our analytical predictions also match fiber network simulations without bending rigidity. (a) To simulate fiber networks, we divide each spring of our original spring networks into $M$ subsprings. We numerically observe (b) a quadratic scaling between critical strain $\gamma^*$ and $\ell_0^* - \ell_0$ (cf. Fig. 4c in the main text), (c) a linear scaling of the shear modulus discontinuity with $\ell_0^* - \ell_0$ (cf. Fig. 4d inset in the main text), (d) the predicted scaling of the relative excess shear modulus beyond the critical strain $\gamma^*$ (cf. Fig. 4d in the main text), and (e) a linear scaling of the shear modulus with the mean rest length for $\gamma = 0$ (cf. Fig. 4f in the main text). (f) Simulations with different values for $M > 1$ lead to quantitatively the same predictions, here shown for the plot in panel e for one of the original spring networks. In panels b-e, we set $M = 4$. In panels b-f, we have used for the original spring network a system size of 128 nodes and a connectivity of $z = 3.2$.

tively independent of the number $M$ as long as $M > 1$ (Fig. S6f). This makes sense, because subspring chains under tension will straighten out and thus have the same effect as the original spring, independent of $M$. Conversely, when replacing springs under compression by a subspring chain, this chain will buckle resulting in a network that behaves as if that subspring chain was not there, independent of $M > 1$. As a consequence of this independence on $M > 1$, the limit $M \to \infty$ is well-defined and corresponds to the behavior of the subspring network with any $M > 1$. Hence, fiber networks without bending rigidity are also faithfully represented by our theory.

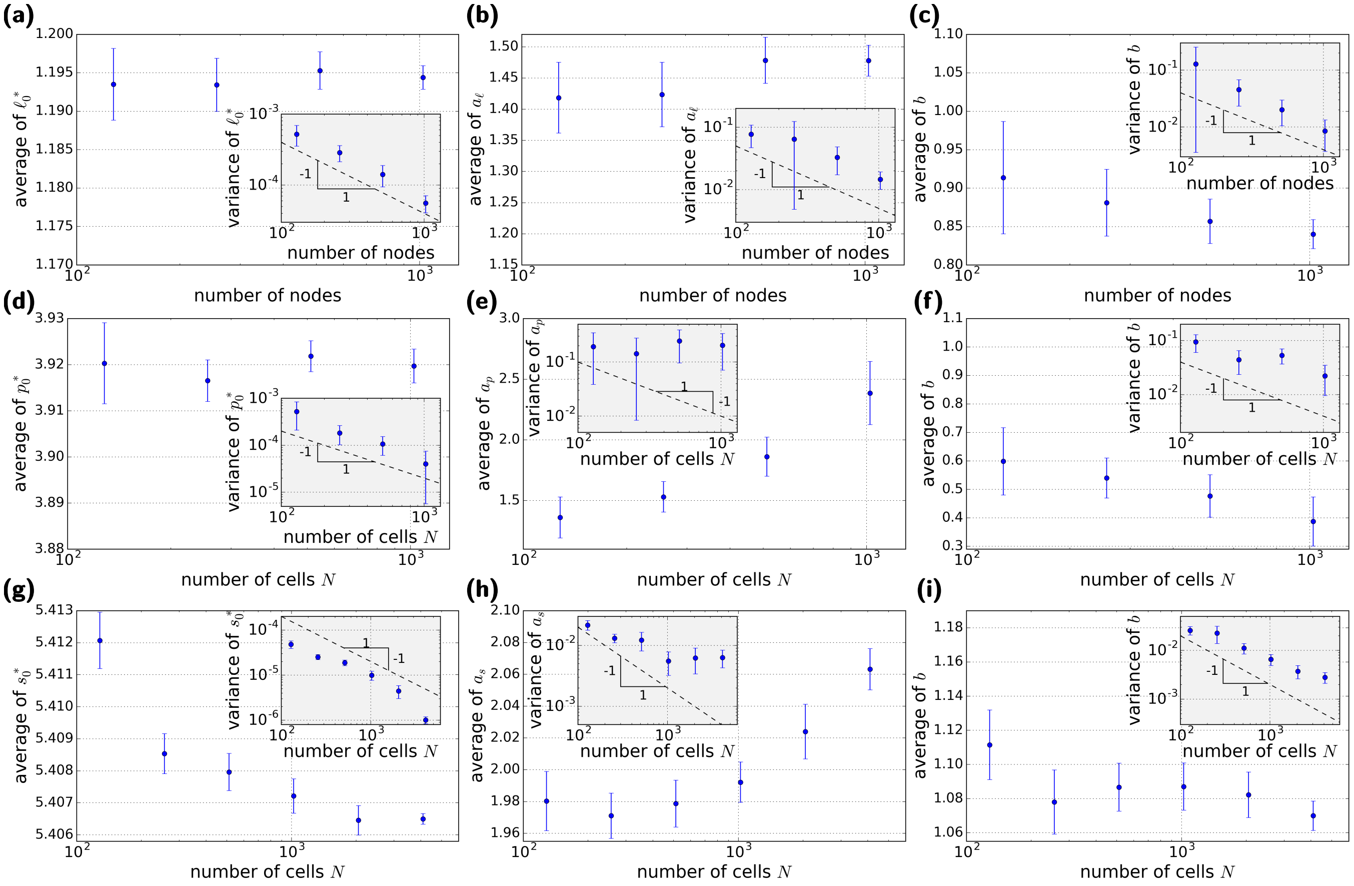


FIG. S7. System-size dependence of the parameters $\ell_0^*$, $a_\ell$, and $b$ characterizing the $\bar{\ell}_{\min}$ function. (a-c) 2D spring networks with $z = 3.2$, (d-f) 2D vertex model with $k_A > 0$, and (g-i) 3D Voronoi model with $k_V > 0$. For the 2D spring networks, all quantities vary only little with system size. The same is also true for the other models with $k_A = 0$. However, we observe a drift in the $a$ and $b$ coefficients for both models with $k_A > 0$.

### D. System-size dependence of the geometric parameters

We also studied the system-size dependence of the parameters $\ell_0^*$, $a_\ell$, $a_a$, and $b$ characterizing the $\ell_{\min}$ function. We find that for all models with $k_A = 0$, the parameters do not depend very strongly on system size (e.g. Fig. S7a-c). At the same time their variances decrease with system size as $\sim 1/N$ (Fig. S7 insets).

In contrast, for models with $k_A > 0$, we find a significant, possibly logarithmic, drift in the coefficients $a_\ell$, both in two and in three dimensions (Fig. S7e,h). At the same time, the variance in $a_\ell$ appears to cease decreasing with system size (Fig. S7 insets to e,h). The coefficients $a_a$ respectively show a very similar behavior (not shown), while the coefficients $b$ appear to possibly also show such a drift albeit somewhat weaker (Fig. S7f,i & insets). We do not yet know where this drift comes from, but we noted that it is much stronger for the 2D vertex model than for the 3D Voronoi model (Fig. S7e,h).

## III. THERE IS AT MOST ONE SELF-STRESS IN THE 2D VERTEX MODEL WITH $k_A = 0$

Here we show analytically that for the $k_A = 0$ case of the 2D vertex model with convex cells, there is at most one self-stress, and that as a consequence the onset of prestresses occurs collectively in *all* cells at once.

For $k_A = 0$, the generalized springs are the $N$ perimeters $p_i$ and the degrees of freedom are the $2N$ vertex positions $\boldsymbol{r}_q$, where $q$ is the vertex index and we assume that all vertices are shared by three cells. Thus, a self-stress in this system is an $N$-dimensional vector $t_i$ with:

$$\sum_i t_i \frac{\partial p_i}{\partial \boldsymbol{r}_q} = 0 \qquad \text{for all vertices } q. \tag{S62}$$

For a given vertex $q$, the partial derivative in the sum is only non-vanishing for the three abutting cells (denoted here by $i, j, k$) such that Eq. (S62) reads for this vertex $q$:

$$t_i \frac{\partial p_i}{\partial \boldsymbol{r}_q} + t_j \frac{\partial p_j}{\partial \boldsymbol{r}_q} + t_k \frac{\partial p_k}{\partial \boldsymbol{r}_q} = 0. \tag{S63}$$

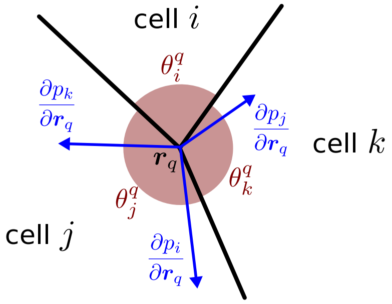


FIG. S8. Definitions of angles for the proof that there is at most one self-stress in the 2D vertex model for $k_A = 0$ (see Section III).

This corresponds to force balance at vertex $q$ with the perimeter tensions $t_i, t_j, t_k$.

With the angles $\theta_i^q, \theta_j^q, \theta_k^q$ between the cell-cell interfaces (Fig. S8), we obtain for the norm of the perimeter derivatives $|\partial p_i/\partial \boldsymbol{r}_q| = 2\cos(\theta_i^q/2)$, and the direction of $\partial p_i/\partial \boldsymbol{r}_q$ is along the angle bisector of $\theta_i^q$ (cf. Fig. S8). If all angles $0 < \theta_i^q < \pi$, then insertion into the force balance equation Eq. (S63) yields

$$\frac{t_i}{\tan(\theta_i^q/2)} = \frac{t_j}{\tan(\theta_j^q/2)} = \frac{t_k}{\tan(\theta_k^q/2)}. \tag{S64}$$

Any solution to Eq. (S62) has to fulfill Eq. (S64) *for each vertex simultaneously*. Thus, in the case where the conditions Eq. (S64) around different vertices are incompatible with each other, there are no nonzero solutions for the $t_i$. In this case there is no self-stress and thus no prestress, i.e. the system is in the floppy regime. If conversely the conditions Eq. (S64) are compatible with each other for all vertices, a nonzero solution for the $t_i$ exists. However, up to a common factor of proportionality, there is only a single solution, because the factors between the $t_i$ for different cells $i$ are uniquely defined by the relations Eq. (S64). Hence, there is at most only one state of self-stress in this model, and the onset of prestresses occurs in *all* cells at once.

## IV. NUMERICAL ENERGY MINIMIZATION

### A. Definitions for shear strain $\gamma$

For all cellular models, we used as definition for the shear strain $\gamma$ the simple shear strain (i.e. in the affine case a change in $\gamma$ corresponds to the displacement $\delta x = y\delta\gamma$ of any point $(x, y)$). For the 2D spring networks, the shear strain $\gamma$ denotes pure shear strain defined such that when starting from a quadratic box, the final box aspect ratio is $\exp(\gamma)$. Note that we expect our results to be independent of whether $\gamma$ denotes simple or pure shear.

### B. 2D spring networks

We initialized the spring networks as packing-derived, randomly cut networks as described in the models section in the main text [9, 15]. To improve the precision as compared to the cellular models, we created our own implementation of the Polak-Ribière version of the conjugate gradient minimization method [16], where for the line searches we use a self-developed Newton method based only on energy derivatives. All states were minimized until the average force per degree of freedom was less than $10^{-12}$. For the $\ell_0$ sweeps (Fig. 1a,b in the main text and Fig. S3a), to prevent switching to a different inherent state, starting from the initial $\ell_0$ value we first decreased $\ell_0$ in steps of 0.01, each time minimizing the energy. These energy minimizations were shear stabilized with respect to the pure shear degree of freedom (i.e. $\gamma$ was allowed to vary during energy minimization) [3]. Afterwards, starting again from the initial configuration, we iteratively increased $\ell_0$ by steps of 0.01.

For the simulations exploring the vicinity of the $(\gamma, \ell_0) = (0, \ell_0^*)$ point (used for the values in Table I, Figs. 2a, 3a, and 4 in the main text, and Fig. S5), we always first looked for the $(\gamma, \ell_0) = (0, \ell_0^*)$ point using a bisection protocol with pure-shear-stabilized minimizations (see also Section I D). We therefore started with the right (floppy) bracket at the initial $\ell_0$ value and the left (rigid) bracket at $\ell_0 = 1.1$, and then executed 25 bisection steps. A configuration was declared rigid whenever the isotropic stress exerted on the boundaries exceeded a value of $10^{-10}$.

We explored the rigid vicinity of the transition point $\ell_0 < \ell_0^*$ (used for Figs. 2a, 3a, and 4c inset,f in the main text, and Fig. S5c) starting from $(\gamma, \ell_0) = (0, \ell_0^*)$ by exponentially increasing $\ell_0^* - \ell_0$ starting from a small initial value, and then each time minimizing the energy *without* shear stabilization to ensure $\gamma = 0$ for these simulations. Similarly, we created the $\gamma$ sweeps for $\ell_0 = \ell_0^*$ (used for Fig. 4e in the main text, and Fig. S5b) by exponentially increasing $\gamma$ starting from $(\gamma, \ell_0) = (0, \ell_0^*)$ and minimizing without shear stabilization.

We explored the boundary between solid and floppy regime (used for Fig. 4c,d inset in the main text, and Fig. S5c) by exponentially increasing $\ell_0 - \ell_0^*$ starting from $(\gamma, \ell_0) = (0, \ell_0^*)$ without shear stabilization. To reduce the switching to different basins, we chopped large $\ell_0$ steps up into smaller steps of 0.01 to include intermittent minimizations. Then, for a given $\ell_0$, we increased $\gamma$ in steps of size 0.001, each time minimizing without shear stabilization. As soon as a rigid state was encountered (isotropic stress on the boundaries exceeds $10^{-10}$), we started a bisection starting from the last rigid and the last floppy states encountered as initial brackets. Using 20 bisection steps, we identified $\gamma^*$. Once $\gamma^*$ was identified, we each time scanned 5 different $\gamma$ values up to 5% above and below $\gamma^*$ to help us verify that there was indeed a discontinuity in the shear modulus. For Fig. 4d in the main text, we explored the rigid vicinity of the transition

more thoroughly using dedicated simulations, where we exponentially increased $\gamma - \gamma^*$ once $\gamma^*$ for $\ell_0 - \ell_0^* = 10^{-4}$ was identified.

### C. 2D vertex model

We always started from Voronoi tessellations of random point patterns, generated using the Computational Geometry Algorithms Library (CGAL, [17]), and we used the BFGS2 implementation of the GNU Scientific Library (GSL, [18]) to minimize the energy. We enforced 3-way vertices and the length cutoff for T1 transitions was set to $10^{-5}$, and there is a maximum possible number of T1 transitions on a single cell-cell interface of $10^4$. For the $p_0$ sweeps, we directly minimized the random initial states (used for Figs. 1c,d in the main text, and Figs. S3b, S4a,b). To reduce the number of networks with prestresses in the floppy regime (cf. Fig. S4b), we removed quadrilaterals from the energy-minimized configurations by repeatedly inducing T1 transitions and minimizing the energy until no quadrilaterals were left. Finally, we discarded simulations that had a total force norm larger than $10^{-5}$, a shear modulus smaller than $-10^{-5}$, or a cell-cell interface with length smaller than the T1 cutoff. To explore the solid vicinity of the transition point (used for the values in Table I, Figs. 2b & inset, 3b in the main text, and Fig. S2a), we proceeded using bisection similar to Ref. [2]. First however, we made sure to exclude quadrilaterals from these states. To this end, we first minimized with $p_0 = 3.99$. Then, we repeatedly induced T1 transitions to remove any quadrilaterals followed by another energy minimization until no quadrilaterals were left. This state at $p_0 = 3.99$ was then the right bracket for the bisection and the left bracket was set to 3.8. Then, we proceeded with the bisection as in Ref. [2] with 18 bisection steps and a shear modulus cutoff of $10^{-8}$. We excluded configurations were the topology (more precisely, the number of neighbors of all cells) changed between the last rigid and floppy states of the bisection, or during the exploration of the solid vicinity of the transition point. All 2D vertex model configurations studied were shear-stabilized with respect to the simple shear degree of freedom.

### D. 2D Voronoi model

We started from random point patterns and minimized the system energy using the BFGS2 routine of the GSL, and we used CGAL to compute the Voronoi tessellations. We discarded simulations that had a total force norm larger than $3 \times 10^{-5}$. For the $p_0$ sweeps, we directly minimized the random initial states (used for Figs. 1c,d in the main text). To explore the solid vicinity of the transition point (used for Table I, Fig. 2b inset in the main text, and Fig. S2a), we proceeded as in Ref. [2] where we started from the initial $p_0$ bracket $[3.7, 3.9]$ and used 20 bisection steps. The cutoff to declare a configuration as rigid was at a shear modulus of $10^{-6}$. To ensure configurations were properly minimized for the exploration of the solid vicinity, we repeated up to 10 minimizations until the force per degree of freedom was smaller than $10^{-8}$. We excluded configurations were the topology (the neighbor number of all cells) changed between the last rigid and floppy states of the bisection, or during the exploration of the solid vicinity of the transition point. Due to limitations of the CGAL library, configurations were not shear stabilized.

### E. 3D Voronoi model

We used the shear-stabilized energy-minimized states generated in Ref. [2] using the BFGS2 multidimensional minimization routine of the GSL, both regarding the $s_0$ sweeps (used for Figs. 1e,f in the main text, and Figs. S3c) as well as the simulations exploring the solid vicinity of the transition point (used for Table I, Figs. 2c & inset, 3c in the main text, and Fig. S2c). To explore the solid vicinity of the transition point for $k_V = 0$, we used slightly different numerical parameters. In particular, the initial bracket for the bisection was $[5.34, 5.40]$, and we performed 13 bisection steps, where a state was considered rigid whenever it had a shear modulus greater than $10^{-6}$.


[1] T C Lubensky, C L Kane, Xiaoming Mao, A Souslov, and Kai Sun, "Phonons and elasticity in critically coordinated lattices," Reports on Progress in Physics **78**, 73901 (2015), arXiv:1503.01324.

[2] Matthias Merkel and M Lisa Manning, "A geometrically controlled rigidity transition in a model for confluent 3D tissues," New Journal of Physics **20**, 022002 (2018).

[3] Simon Dagois-Bohy, Brian P. Tighe, Johannes Simon, Silke Henkes, and Martin Van Hecke, "Soft-sphere packings at finite pressure but unstable to shear," Physical Review Letters **109**, 1–5 (2012), arXiv:1203.3364.

[4] Dapeng Bi, J. H. Lopez, J. M. Schwarz, and M. Lisa Manning, "A density-independent rigidity transition in biological tissues," Nature Physics **11**, 1074–1079 (2015), arXiv:1409.0593.

[5] Nebojsa Murisic, Vincent Hakim, Ioannis G. Kevrekidis, Stanislav Y. Shvartsman, and Basile Audoly, "From Discrete to Continuum Models of Three-Dimensional Deformations in Epithelial Sheets," Biophysical Journal **109**, 154–163 (2015).

[6] Xingbo Yang, Dapeng Bi, Michael Czajkowski, Matthias Merkel, M. Lisa Manning, and M. Cristina Marchetti, "Correlating Cell Shape and Cellular Stress in

Motile Confluent Tissues," Proceedings of the National Academy of Sciences **114**, 12663–12668 (2017), arXiv:1704.05951.

[7] Daniel Marc Sussman and Matthias Merkel, "No unjamming transition in a Voronoi model of biological tissue," Soft Matter (2018), 10.1039/C7SM02127E, arXiv:1708.03396.

[8] Brian P. Tighe, "Relaxations and rheology near jamming," Physical Review Letters **107**, 1–5 (2011), arXiv:1106.0714v2.

[9] Karsten Baumgarten and Brian P. Tighe, "Normal Stresses, Contraction, and Stiffening in Sheared Elastic Networks," Physical Review Letters **120**, 148004 (2018).

[10] E. Lerner, G. During, and M. Wyart, "A unified framework for non-Brownian suspension flows and soft amorphous solids," Proceedings of the National Academy of Sciences **109**, 4798–4803 (2012), arXiv:1112.0558.

[11] Gustavo Düring, Edan Lerner, and Matthieu Wyart, "Phonon gap and localization lengths in floppy materials," Soft Matter **9**, 146–154 (2013), arXiv:1204.3542.

[12] Karsten Baumgarten, *to be published*, Ph.D. thesis, Delft University of Technology (2018).

[13] A. S. Lodge and J. Meissner, "On the use of instantaneous strains, superposed on shear and elongational flows of polymeric liquids, to test the Gaussian network hypothesis and to estimate the segment concentration and its variation during flow," Rheologica Acta **11**, 351–352 (1972).

[14] Anne S. G. van Oosten, Mahsa Vahabi, Albert J Licup, Abhinav Sharma, Peter A Galie, Fred C. MacKintosh, and Paul A Janmey, "Uncoupling shear and uniaxial elastic moduli of semiflexible biopolymer networks: compression-softening and stretch-stiffening," Scientific Reports **6**, 19270 (2016).

[15] M. Wyart, H. Liang, A. Kabla, and L. Mahadevan, "Elasticity of floppy and stiff random networks," Physical Review Letters **101**, 1–4 (2008), arXiv:0806.4571v1.

[16] Stephen G Nash and Ariela Sofer, *Linear and Nonlinear Programming* (McGraw-Hill College, 1995).

[17] `https://www.cgal.org/`.

[18] `https://gnu.org/software/gsl/`.
